# Supplementary material for: Transform-Dependent Adversarial Attacks
Source: arXiv:2406.08443 source file (2025-03-10)
Supplement: Supplementary file 1 [file tab-cls-def.tex]

\begin{table*}[]

\centering
\small
\caption{Evaluation results of transformation-dependent attack against input transformation defenses. Each column reports the best ASR of transform-dependent adversaries that can provide with any transform parameter. Row \textit{Random} reporting transform parameter for defense transformations is randomly sampled as $S \sim [0.5, 2.0]$, $\gamma \sim [0.5, 2.0]$, $Q \sim [10, 90]$ and $\sigma \sim [0.5, 3.0]$ for scaling, gamma, JPEG and blurring transformation as defense. Average over 6 models.}
\label{tab:cls-def}

\begin{tabular}{cccccccccc}
\hline
\multicolumn{1}{c|}{\multirow{2}{*}{\begin{tabular}[c]{@{}c@{}}Scaling\\ factor\end{tabular}}} & \multicolumn{4}{c|}{\begin{tabular}[c]{@{}c@{}}Scaling as defense, ASR(\%) $\uparrow$\end{tabular}} & \multicolumn{1}{c|}{\multirow{2}{*}{\begin{tabular}[c]{@{}c@{}}Gamma\\ value\end{tabular}}} & \multicolumn{4}{c}{\begin{tabular}[c]{@{}c@{}}Gamma as defense, ASR(\%) $\uparrow$\end{tabular}} \\
\multicolumn{1}{c|}{} & \textbf{Scale} & Blur & Gamma & \multicolumn{1}{c|}{JPEG} & \multicolumn{1}{c|}{} & Scale & Blur & \textbf{Gamma} & JPEG \\ \hline
\multicolumn{1}{c|}{$S=0.5$} & 89.60 & 0.10 & 0.30 & \multicolumn{1}{c|}{0.10} & \multicolumn{1}{c|}{$\gamma=0.5$} & 73.10 & 60.20 & 76.70 & 2.70 \\
\multicolumn{1}{c|}{$S=1.5$} & 99.40 & 0.30 & 0.30 & \multicolumn{1}{c|}{0.20} & \multicolumn{1}{c|}{$\gamma=2.0$} & 45.90 & 28.60 & 35.60 & 3.20 \\
\multicolumn{1}{c|}{Random} & 88.62 & 0.50 & 1.40 & \multicolumn{1}{c|}{0.10} & \multicolumn{1}{c|}{Random} & 68.80 & 78.90 & 85.20 & 47.30 \\ \hline
\multicolumn{1}{c|}{Average} & \textbf{92.45} & 0.30 & 0.67 & \multicolumn{1}{c|}{0.13} & \multicolumn{1}{c|}{Average} & 62.60 & 55.90 & \textbf{65.83} & 17.73 \\ \hline
\multicolumn{10}{l}{} \\ \hline
\multicolumn{1}{c|}{\multirow{2}{*}{\begin{tabular}[c]{@{}c@{}}Compression\\ quality\end{tabular}}} & \multicolumn{4}{c|}{\begin{tabular}[c]{@{}c@{}}JPEG as defense, ASR(\%) $\uparrow$\end{tabular}} & \multicolumn{1}{c|}{\multirow{2}{*}{\begin{tabular}[c]{@{}c@{}}Standard\\ deviation\end{tabular}}} & \multicolumn{4}{c}{\begin{tabular}[c]{@{}c@{}}Blurring as defense, ASR(\%) $\uparrow$\end{tabular}} \\
\multicolumn{1}{c|}{} & Scale & Blur & Gamma & \multicolumn{1}{c|}{\textbf{JPEG}} & \multicolumn{1}{c|}{} & Scale & \textbf{Blur} & Gamma & JPEG \\ \hline
\multicolumn{1}{c|}{$Q=20$} & 1.10 & 0.60 & 0.20 & \multicolumn{1}{c|}{82.20} & \multicolumn{1}{c|}{$\sigma=0.5$} & 87.30 & 95.80 & 91.40 & 28.40 \\
\multicolumn{1}{c|}{$Q=50$} & 17.10 & 13.10 & 0.20 & \multicolumn{1}{c|}{95.40} & \multicolumn{1}{c|}{$\sigma=1.5$} & 8.50 & 32.50 & 0.30 & 0.40 \\
\multicolumn{1}{c|}{$Q=80$} & 69.40 & 63.30 & 1.90 & \multicolumn{1}{c|}{98.10} & \multicolumn{1}{c|}{$\sigma=3.0$} & 2.50 & 14.30 & 0.10 & 0.10 \\
\multicolumn{1}{c|}{Random} & 24.10 & 22.60 & 1.10 & \multicolumn{1}{c|}{33.70} & \multicolumn{1}{c|}{Random} & 20.60 & 37.50 & 3.80 & 1.90 \\ \hline
\multicolumn{1}{c|}{Average} & 27.93 & 24.90 & 0.85 & \multicolumn{1}{c|}{\textbf{77.35}} & \multicolumn{1}{c|}{Average} & 29.73 & \textbf{45.03} & 23.90 & 7.70 \\ \hline
\end{tabular}

\end{table*}
