# Supplementary material for: Transform-Dependent Adversarial Attacks
Source: arXiv:2406.08443 source file (2025-03-10)
Supplement: Supplementary file 2 [file tab-cls-rob-acc.tex]

\begin{table*}[h]

\centering
\small
\caption{Robust models evaluation with only transformation. The column labeled \textit{Original} presents model accuracy for the original images (i.e., $f(\mathbf{x})$). The column \textit{Transformed} evaluate models accuracy after image transformations (i.e., $f(T(\mathbf{x};\theta))$).}

\label{tab:attack-rob-acc}

\begin{tabular}{ccccccc}
\hline
\multicolumn{1}{c|}{\multirow{3}{*}{Model}} & \multicolumn{3}{c|}{Scaling} & \multicolumn{3}{c}{Blurring} \\ \cline{2-7} 
\multicolumn{1}{c|}{} & \multicolumn{1}{c|}{Original} & \multicolumn{2}{c|}{Transformed} & \multicolumn{1}{c|}{Original} & \multicolumn{2}{c}{Transformed} \\
\multicolumn{1}{c|}{} & \multicolumn{1}{c|}{$S=1.0$} & $S=0.5$ & \multicolumn{1}{c|}{$S=1.5$} & \multicolumn{1}{c|}{(no blur)} & $\sigma=0.5$ & $\sigma=1.5$ \\ \hline
\multicolumn{1}{c|}{ResNet-50} & \multicolumn{1}{c|}{100.0} & 69.20 & \multicolumn{1}{c|}{90.40} & \multicolumn{1}{c|}{100.0} & 95.80 & 76.50 \\
\multicolumn{1}{c|}{ResNet-50-eps4} & \multicolumn{1}{c|}{100.0} & 35.40 & \multicolumn{1}{c|}{65.20} & \multicolumn{1}{c|}{100.0} & 88.10 & 52.90 \\
\multicolumn{1}{c|}{ResNet-50-eps8} & \multicolumn{1}{c|}{100.0} & 32.00 & \multicolumn{1}{c|}{61.30} & \multicolumn{1}{c|}{100.0} & 85.90 & 53.00 \\ \hline
\multicolumn{1}{c|}{Average} & \multicolumn{1}{c|}{100.0} & 45.53 & \multicolumn{1}{c|}{72.30} & \multicolumn{1}{c|}{100.0} & 89.93 & 60.80 \\ \hline
\multicolumn{7}{l}{} \\ \hline
\multicolumn{1}{c|}{\multirow{3}{*}{Model}} & \multicolumn{3}{c|}{Gamma} & \multicolumn{3}{c}{JPEG} \\ \cline{2-7}
\multicolumn{1}{c|}{} & \multicolumn{1}{c|}{Original} & \multicolumn{2}{c|}{Transformed} & \multicolumn{1}{c|}{Original} & \multicolumn{2}{c}{Transformed} \\
\multicolumn{1}{c|}{} & \multicolumn{1}{c|}{$\gamma=1.0$} & $\gamma=0.5$ & \multicolumn{1}{c|}{$\gamma=2.0$} & \multicolumn{1}{c|}{$Q=100$} & $Q=50$ & $Q=80$ \\ \hline
\multicolumn{1}{c|}{ResNet-50} & \multicolumn{1}{c|}{100.0} & 92.30 & \multicolumn{1}{c|}{90.70} & \multicolumn{1}{c|}{100.0} & 86.50 & 91.30 \\
\multicolumn{1}{c|}{ResNet-50-eps4} & \multicolumn{1}{c|}{100.0} & 43.90 & \multicolumn{1}{c|}{35.10} & \multicolumn{1}{c|}{100.0} & 88.00 & 91.30 \\
\multicolumn{1}{c|}{ResNet-50-eps8} & \multicolumn{1}{c|}{100.0} & 38.10 & \multicolumn{1}{c|}{31.20} & \multicolumn{1}{c|}{100.0} & 88.40 & 92.50 \\ \hline
\multicolumn{1}{c|}{Average} & \multicolumn{1}{c|}{100.0} & 58.10 & \multicolumn{1}{c|}{52.33} & \multicolumn{1}{c|}{100.0} & 87.63 & 91.70 \\ \hline
\end{tabular}

\end{table*}
