# Supplementary material for: Transform-Dependent Adversarial Attacks
Source: arXiv:2406.08443 source file (2025-03-10)
Supplement: Supplementary file 3 [file tab-cls-bb-1.tex]

\begin{table*}[]

\centering
\small
\caption{Blackbox transfer evaluation for scaling and blurring-dependent adversarial examples. Diagonal entries are whitebox attacks.
Higher value indicates better attack performance.
Adversaries are generated with untargeted attack optimization.
The perturbation budget is $\|\delta\|_\infty \leq 10$.
}
\label{tab:attack-bb-1}

\begin{tabular}{ccccccc}
\hline
\multicolumn{1}{c|}{\multirow{2}{*}{Surrogate}} & \multicolumn{6}{c}{Scaling, blackbox ASR (\%) $\uparrow$} \\
\multicolumn{1}{c|}{} & VGG-19 & ResNet-50 & Dense-161 & Inc-v3 & ViT-L-16 & ViT-L-32 \\ \hline
\multicolumn{1}{c|}{VGG-19} & 100.0 & 38.10 & 44.30 & 73.60 & 16.10 & 23.40 \\
\multicolumn{1}{c|}{ResNet-50} & 44.60 & 99.90 & 46.70 & 74.20 & 15.50 & 23.20 \\
\multicolumn{1}{c|}{Dense-161} & 45.40 & 39.80 & 99.90 & 74.00 & 15.40 & 23.80 \\
\multicolumn{1}{c|}{Inc-v3} & 42.80 & 35.30 & 43.00 & 98.70 & 16.20 & 22.50 \\
\multicolumn{1}{c|}{ViT-L-16} & 43.40 & 37.50 & 43.60 & 72.70 & 94.20 & 25.00 \\
\multicolumn{1}{c|}{ViT-L-32} & 44.30 & 38.90 & 44.00 & 74.40 & 17.70 & 90.70 \\ \hline
\multicolumn{1}{c|}{Average} & 53.42 & 48.25 & 53.58 & 77.93 & 29.18 & 34.77 \\ \hline
\multicolumn{7}{l}{} \\ \hline
\multicolumn{1}{c|}{\multirow{2}{*}{Surrogate}} & \multicolumn{6}{c}{Blurring, blackbox ASR (\%) $\uparrow$} \\
\multicolumn{1}{c|}{} & VGG-19 & ResNet-50 & Dense-161 & Inc-v3 & ViT-L-16 & ViT-L-32 \\ \hline
\multicolumn{1}{c|}{VGG-19} & 100.0 & 28.70 & 28.10 & 44.00 & 17.20 & 24.30 \\
\multicolumn{1}{c|}{ResNet-50} & 38.70 & 99.90 & 30.40 & 45.10 & 18.00 & 25.00 \\
\multicolumn{1}{c|}{Dense-161} & 38.90 & 31.40 & 99.90 & 44.90 & 17.80 & 24.70 \\
\multicolumn{1}{c|}{Inc-v3} & 34.90 & 26.60 & 25.10 & 98.40 & 17.10 & 23.30 \\
\multicolumn{1}{c|}{ViT-L-16} & 36.90 & 30.20 & 28.30 & 43.90 & 97.90 & 27.30 \\
\multicolumn{1}{c|}{ViT-L-32} & 35.50 & 31.00 & 28.20 & 44.10 & 20.80 & 94.70 \\ \hline
\multicolumn{1}{c|}{Average} & 47.48 & 41.30 & 40.00 & 53.40 & 31.47 & 36.55  \\ \hline
\end{tabular}

\end{table*}
