# Supplementary material for: Transform-Dependent Adversarial Attacks
Source: arXiv:2406.08443 source file (2025-03-10)
Supplement: Supplementary file 4 [file tab-cls-bb-2.tex]

\begin{table*}[]

\centering
\small
\caption{
Blackbox transfer evaluation for gamma and compression-dependent adversarial examples. Diagonal entries are whitebox attacks.
Higher value indicates better attack performance.
Adversaries are generated with untargeted attack optimization.
The perturbation budget is $\|\delta\|_\infty \leq 10$.
}
\label{tab:attack-bb-2}

\begin{tabular}{ccccccc}
\hline
\multicolumn{1}{c|}{\multirow{2}{*}{Surrogate}} & \multicolumn{6}{c}{Gamma, blackbox ASR (\%) $\uparrow$} \\
\multicolumn{1}{c|}{} & VGG-19 & ResNet-50 & Dense-161 & Inc-v3 & ViT-L-16 & ViT-L-32 \\ \hline
\multicolumn{1}{c|}{VGG-19} & 100.0 & 18.80 & 14.00 & 35.80 & 14.00 & 19.40 \\
\multicolumn{1}{c|}{ResNet-50} & 25.10 & 100.00 & 17.90 & 36.30 & 13.40 & 19.80 \\
\multicolumn{1}{c|}{Dense-161} & 26.50 & 24.60 & 100.0 & 39.10 & 14.20 & 19.40 \\
\multicolumn{1}{c|}{Inc-v3} & 21.00 & 19.90 & 14.10 & 99.70 & 14.40 & 19.30 \\
\multicolumn{1}{c|}{ViT-L-16} & 23.90 & 21.20 & 16.50 & 37.70 & 99.30 & 20.80 \\
\multicolumn{1}{c|}{ViT-L-32} & 24.50 & 19.70 & 15.30 & 36.30 & 14.90 & 99.20 \\ \hline
\multicolumn{1}{c|}{Average} & 36.83 & 34.03 & 29.63 & 47.48 & 28.37 & 32.98 \\ \hline
\multicolumn{7}{l}{} \\ \hline
\multicolumn{1}{c|}{\multirow{2}{*}{Surrogate}} & \multicolumn{6}{c}{JPEG, blackbox ASR (\%) $\uparrow$} \\
\multicolumn{1}{c|}{} & VGG-19 & ResNet-50 & Dense-161 & Inc-v3 & ViT-L-16 & ViT-L-32 \\ \hline
\multicolumn{1}{c|}{VGG-19} & 99.70 & 28.10 & 21.70 & 39.00 & 20.90 & 18.80 \\
\multicolumn{1}{c|}{ResNet-50} & 40.80 & 98.50 & 25.30 & 39.30 & 20.70 & 18.90 \\
\multicolumn{1}{c|}{Dense-161} & 40.50 & 32.40 & 98.30 & 40.60 & 21.10 & 19.70 \\
\multicolumn{1}{c|}{Inc-v3} & 34.10 & 26.70 & 20.90 & 95.40 & 20.70 & 18.80 \\
\multicolumn{1}{c|}{ViT-L-16} & 34.30 & 27.30 & 21.50 & 37.20 & 92.00 & 19.70 \\
\multicolumn{1}{c|}{ViT-L-32} & 35.80 & 28.40 & 21.70 & 36.50 & 22.90 & 92.70 \\ \hline
\multicolumn{1}{c|}{Average} & 47.53 & 40.23 & 34.90 & 48.00 & 33.05 & 31.43  \\ \hline
\end{tabular}

\end{table*}
