# Supplementary material for: Transform-Dependent Adversarial Attacks
Source: arXiv:2406.08443 source file (2025-03-10)
Supplement: Supplementary file 6 [file tab-cls-rob-mis.tex]

\begin{table}[h]

\centering
\small
\caption{Robust models consistency rate (\%). We generate attacks for each ResNet50 model and provide evaluation of models consistency rate for perturbed image without any transformation applied.}

\begin{tabular}{c|ccc}
\hline
\multirow{2}{*}{\begin{tabular}[c]{@{}c@{}}Perturbation\\ budget\end{tabular}} & \multicolumn{3}{c}{Classifier model} \\
 & ResNet50 & ResNet50-eps4 & ResNet50-eps8 \\ \hline
$\varepsilon=4$ & 1.30 & 84.33 & 87.10 \\
$\varepsilon=8$ & 0.00 & 74.67 & 83.23 \\ \hline
\end{tabular}

\label{tab:attack-rob-mis}

\end{table}
