# Supplementary material for: Transform-Dependent Adversarial Attacks
Source: arXiv:2406.08443 source file (2025-03-10)
Supplement: Supplementary file 7 [file supp.tex]

\newpage
\clearpage


\begin{strip} 
    \begin{center} 
        {\Large  \textbf{Transform-Dependent Adversarial Attacks \\ (Supplementary Material)}}
    \end{center} 
\end{strip} 



\newcommand{\beginsupplement}{%
        \setcounter{table}{0}
        \renewcommand{\thetable}{S\arabic{table}}%
        \setcounter{figure}{0}
        \renewcommand{\thefigure}{S\arabic{figure}}%
        \setcounter{section}{0}
        \renewcommand{\thesection}{S\arabic{section}}%
}
\makeatletter
\newcommand\refwithdefault[2]{%
  \@ifundefined{r@#1}{%
    #2%
  }{%
    \ref{#1}%
  }%
}
\makeatother



\section*{Summary}

In this supplementary material, we present additional evaluation results for various models (both original and robustified) with images subjected to diverse transformations 
(corresponding to Sec.~\textcolor{red}{4.2} and Sec.~\textcolor{red}{4.4} in the main paper).
% (corresponding to \cref{subsec:whitebox} and \cref{sec:rob} in the main paper).
%
We also present additional results demonstrating the efficacy of our attacks against adversarial training. Moreover, we illustrate the adaptability of our attacks to different transformation types, accompanied by additional evaluations in more challenging attack scenarios. Lastly, we include supplementary visualizations of adversarial examples to facilitate qualitative assessment.


% \appendix
\beginsupplement

\section{Accuracy evaluations} 


In \cref{subsec:whitebox} of our main paper, we presented targeted attacks crafted to exploit vulnerabilities specific to scaling, blurring, gamma correction, and JPEG compression transformations. We assess the Attack Success Rate (ASR) on a wide range of models: \{VGG-19-BN, ResNet50, DenseNet-121, InceptionV3, ViT-L-16, ViT-L-32\}. Our objective here is to clarify that the adversarial effects we observe are not merely the result of image transformations but are indicative of deeper vulnerabilities introduced by our adversarial perturbations. \cref{tab:cls-acc} provides model classification accuracy for clean images that have undergone the same transformations we employ in our attack generation process. This comparison reveals varying degrees of sensitivity among the models to different transformations. Interestingly, while most models demonstrate robust performance (e.g., over 80\% accuracy) on transformed but clean images, older architectures like InceptionV3 show a marked vulnerability. Specifically, the accuracy for InceptionV3 drops significantly to 69.70\% under these conditions, highlighting a comparative lack of robustness to transformations. Our experiment underscores the evolving nature of model robustness, where newer architectures like ViT-L-16 and ViT-L-32 manage to maintain high accuracy despite transformations that significantly impact older models like VGG and InceptionV3. Nevertheless, all models are highly vulnerable to our transform-dependent attacks.



\input{tables/supp/tab-cls-acc}
\input{tables/supp/tab-cls-rob-acc}
\input{tables/supp/tab-cls-rob-mis}

\section{Attacks against robust models}
In \cref{subsec:robust} of the main paper, we demonstrate the effectiveness of transform-dependent attacks in deceiving adversarially-trained robust models. Here, we extend our analysis by providing comprehensive evaluations for such robust models.

In addition to the experiments detailed in Table~\textcolor{red}{5}, which underscore the susceptibility of robust models to misclassifications induced by our attacks, we delve deeper into their performance under various transformations, as outlined in \cref{tab:attack-rob-acc}. Given that robustified models exhibit diminished accuracy even on clean images, our focus shifts to evaluating the ``consistency" of predictions before and after transformations. Specifically, we assess consistency by examining whether instances satisfy $f(\mathbf{x})=f(T(\mathbf{x};\theta))$.

Each column labeled \textit{Transformed} in \cref{tab:attack-rob-acc} reports the prediction consistency of images in their original form (i.e., the percentage of times $f(\mathbf{x})=f(T(\mathbf{x};\theta))$). Notably, all values for columns labeled \textit{Original} are $100\%$ since the prediction for an image without any transformation remains identical to the original condition. However, in the \textit{Transformed} columns, we observe that the non-robust ResNet50 exhibits greater resilience to distribution shift introduced by image transformations compared to ResNet50-eps4 and ResNet50-eps8.

For reference, we include a model consistency evaluation for both clean and perturbed images under the original condition (i.e., without any transformation involved in the attack) in \cref{tab:attack-rob-mis}. Notably, while facing attacks, the non-robust ResNet50 fails to provide consistent predictions, whereas robust models maintain consistent predictions with a consistency rate exceeding $80\%$ on average.

Our findings underscore that traditional adversarial training falls short in effectively countering our attacks, as it entails a trade-off between in-distribution adversarial robustness and out-of-distribution generalization to transformed images. 


\input{tables/supp/tab-cls-adapt}
\section{Adapt other optimization methods}
In experiments of our main paper, we mainly focus on solving transform-dependent attacks using PGD~\cite{madry2017towards}. In principle, our attacks can also be generated with other optimization methods. Here we provide results of transform-dependent attacks adaption with some commonly used methods, including FGSM~\cite{goodfellow2014explaining}, MIM~\cite{dong2018boosting}, C\&W~\cite{carlini2017towards}, and make a comparison to PGD results presented in the main text experiment.

%
We present the average ASR for scale-dependent targeted attacks (under same setting as \cref{tab:cls-asr} in main text) in \cref{tab:attack-adapt}. MIM, C\&W, and PGD are iterative methods and offer high ASR but the single-step FGSM is insufficient to solve transform-dependent attacks.





\section{More transformations}
In addition to the transformations demonstrated in the main paper, 
Sec.~\textcolor{red}{4.1} (scaling, blurring, gamma, and JPEG), we extend transform-dependent attacks to two more geometric transformations --- flipping and perspective transformations.





\subsection{Flip-dependent attack}

In our examination of flip-dependent attacks, we explore three specific targeted scenarios designed to activate upon the network's receipt of images subjected to vertical flip, horizontal flip, and no flip (retaining their original orientation) as inputs. The findings, as detailed in ~\cref{tab:attack-flip}, reveal a notable efficacy of these flip-dependent attacks, achieving an ASR of 90\% across the majority of evaluated models.


\input{tables/supp/tab-cls-flip}
\input{tables/supp/tab-cls-persp}



\subsection{Perspective-dependent attack}

Here, we introduce perspective-dependent attacks to mimic the variability encountered when taking photos from different angles. We categorize these variations into three predefined perspectives: viewing the subject from the front, from above, and from below, labeled as perspectives 1, 2, and 3, respectively. Specifically, perspective 1 maintains the image in its original state, illustrating a front-facing viewpoint. Perspective 2 simulates a downward view by transforming the image axis from \{(0,0), (223,0)\} to \{(56,56), (168,56)\}, and perspective 3 simulates an upward view by altering the image axis from \{(0,223), (223,223)\} to \{(56,168), (168,168)\}.

The results, as noted in ~\cref{tab:attack-perspe}, demonstrate the effectiveness of these perspective-dependent attacks, with targeted strategies achieving an overall ASR of over 90\% when images are presented from these varied perspectives.



\section{More challenging attack targets}
\input{tables/supp/tab-cls-hard}

In \cref{subsec:whitebox} 
%
of the main paper, we initially employed a random selection process to choose three distinct classes from the set of $1000$ ImageNet classes as our target labels, denoted as $\{y_i^\star\}_{i=1}^3$. Here, we maintain consistency with our attack settings and classification models, but instead of random selection, we opt to target the \textit{three least-likely labels} extracted from the probability vectors.

In this continuation, we evaluate the Adversarial Success Rate (ASR) under these modified attack settings, as presented in \cref{tab:attack-hard}. This evaluation demonstrates the efficacy of our attack formulation even when faced with the challenge of targeting the least-likely labels. 



% \section{Memory and computation resources. } We used a single {NVIDIA RTX 2080Ti (12 GB)} for all the experiments. Average times for generating $\{3,5,10\}$ target attacks are $\{2.61, 4.29, 8.67\}$ sec/image.


\section{More visual examples}
For enhanced qualitative evaluation, we offer additional visual examples showcasing successful transform-dependent adversarial instances against image classification models in~\cref{fig:cls-supp-1} and \cref{fig:cls-supp-2}. Moreover, we present further examples of selective hiding attacks targeting object detection models in~\cref{fig:det-supp-1}, \cref{fig:det-supp-2}, and~\cref{fig:det-supp-3}.

The examples in~\cref{fig:cls-supp-1} and \cref{fig:cls-supp-2} illustrate that with imperceptible noise perturbation, an image can be misclassified as multiple target labels when subjected to specific image transformations.

In the case of selective hiding attacks, consider the images in the first row of \cref{fig:det-supp-1} as an illustration. It demonstrates that in the clean image, objects labeled as three distinct categories (\textit{person, ski}, and \textit{snowboard}) are detected. However, upon adding scale-dependent perturbations, objects labeled as one of these categories become hidden in three differently scaled versions of perturbed images, as depicted in the titles: \textit{$0.5\times$ --- Hide "person"}, \textit{$1.0\times$ --- Hide "ski"}, and \textit{$1.5\times$ --- Hide "snowboard"}.



\input{figures/supp/vis-cls-supp-1}
\input{figures/supp/vis-cls-supp-2}
\input{figures/supp/vis-det-supp-1}
\input{figures/supp/vis-det-supp-2}
\input{figures/supp/vis-det-supp-3}
